# Supplementary material for: A density-fitting implementation of the density-based basis-set correction method
Source: arXiv:2309.10390 source file (2024-02-19)
Supplement: Supplementary file 1 [file supp_info.pdf]

# Supplementary Material for “A density-fitting implementation of the density-based basis-set correction method”

Andreas Heßelmann,<sup>1,\*</sup> Emmanuel Giner,<sup>2,†</sup> Peter Reinhardt,<sup>2,‡</sup> Peter  
J. Knowles,<sup>3,§</sup> Hans-Joachim Werner,<sup>1,¶</sup> and Julien Toulouse<sup>2,4,\*\*</sup>

<sup>1</sup>*Institute for Theoretical Chemistry, University of Stuttgart, 70569, Stuttgart, Germany*

<sup>2</sup>*Laboratoire de Chimie Théorique, Sorbonne Université and CNRS, F-75005 Paris, France*

<sup>3</sup>*School of Chemistry, Cardiff University, Cardiff CF10 3AT, United Kingdom*

<sup>4</sup>*Institut Universitaire de France, F-75005 Paris, France*

(Dated: December 11, 2023)

## I. COMPUTATION TIMES FOR THE DFT-BASED BASIS-SET CORRECTION

Table I reports computation times for calculating the PBE-based basis-set correction for four molecules. Three methods for dealing with the two-electron integrals are compared: conventional (when possible), integral-direct, and density fitting. The integral-direct integral transformation used is from the CCSD program described in Ref. 1. This also computes the integrals ( $ijklab$ ) as well as a Fock matrix, which are not needed for the basis-set correction. The 3-index integrals in the density-fitting calculations are computed without symmetry. Only valence orbitals have been included in the basis-set correction calculations. The spatial grid threshold is 1d-6 (default).

The density-fitting algorithm scales formally as  $O(N^4)$ , while the conventional and integral-direct methods scale as  $O(N^5)$ , where  $N$  is a measure of the molecular size (e.g. the number of electrons  $N_{\text{el}}$  or the number of basis functions  $N_{\text{basis}}$  - not the spatial size). Taking the number of basis functions as measure of size, the scaling exponents obtained from the timings of last 2 molecules are:

density fitting (parallel) : 1.84,

density fitting (serial) : 3.45,

integral-direct (parallel) : 4.56,

integral-direct (serial) : 5.13,

quite as expected. In the last integral-direct calculation the computation of the integrals took 771 seconds and the assembly of the basis-set correction 247 seconds (using 16 cores).

---

\*Electronic address: andreas.hesselmann@theochem.uni-stuttgart.de

†Electronic address: emmanuel.giner@lct.jussieu.fr

‡Electronic address: peter.reinhardt@lct.jussieu.fr

§Electronic address: KnowlesPJ@Cardiff.ac.uk

¶Electronic address: werner@theochem.uni-stuttgart.de

\*\*Electronic address: toulouse@lct.jussieu.fr

TABLE I: Elapsed times (in seconds) for computing the PBE-based basis-set correction with the aug-cc-pVTZ basis set. The number of basis functions  $N_{\text{basis}}$  is reported. The calculations were performed on an Intel Xeon CPU E5-2660 v3@2.60GHz.

| Molecule (symmetry)          | $N_{\text{basis}}$ | method          | serial | parallel <sup>a</sup> |
|------------------------------|--------------------|-----------------|--------|-----------------------|
| urea ( $C_2$ )               | 276                | conventional    | 11.0   | 2.6                   |
|                              |                    | integral-direct | 38.3   | 4.3                   |
|                              |                    | density fitting | 5.9    | 2.5                   |
| benzene ( $D_{2h}$ )         | 414                | conventional    | 7.7    | 1.4                   |
|                              |                    | integral-direct | 96.7   | 12.6                  |
|                              |                    | density fitting | 10.3   | 6.3                   |
| n-hexane ( $C_1$ )           | 598                | integral-direct | 1615.5 | 145.4                 |
|                              |                    | density fitting | 86.8   | 22.2                  |
| tetramethylpentane ( $C_1$ ) | 874                | integral-direct | 9128.8 | 1020.4                |
|                              |                    | density fitting | 321.1  | 44.6                  |

<sup>a</sup>Using 16 MPI processes.

## II. FURTHER STATISTICAL MEASURES ON THE FH51 SET

Table II reports mean errors, standard deviations and maximal absolute errors in reaction energies of the FH51 set with respect to MP2/CBS with *avnz* basis sets. For all the different density-functional approximations except for LYP, the main effect of the basis-set correction is to systematically reduce the standard deviation and maximal absolute error obtained at the uncorrected MP2 level.

TABLE II: Mean error (ME), standard deviation (SD), and maximal absolute error (MAX) (in kcal/mol) in reaction energies of the FH51 set with respect to MP2/CBS with *avnz* basis sets. The MP2/CBS reference is estimated as MP2-F12/av5z.

|                                | ME    |       |       |       | SD   |      |      |      | MAX   |      |      |      |
|--------------------------------|-------|-------|-------|-------|------|------|------|------|-------|------|------|------|
|                                | avdz  | avtz  | avqz  | av5z  | avdz | avtz | avqz | av5z | avdz  | avtz | avqz | av5z |
| MP2                            | -0.52 | 0.09  | 0.01  | 0.01  | 3.11 | 1.03 | 0.40 | 0.20 | 12.61 | 3.82 | 1.59 | 0.73 |
| MP2+CABS                       | 0.09  | 0.02  | 0.01  | 0.01  | 1.27 | 0.74 | 0.32 | 0.17 | 3.42  | 2.20 | 0.98 | 0.54 |
| MP2+PBE                        | -0.93 | -0.07 | -0.08 | -0.03 | 2.32 | 0.50 | 0.17 | 0.06 | 8.43  | 1.88 | 0.59 | 0.19 |
| MP2+CABS+PBE                   | -0.32 | -0.14 | -0.08 | -0.03 | 0.87 | 0.25 | 0.11 | 0.05 | 3.00  | 1.05 | 0.35 | 0.17 |
| MP2+CABS+LDA                   | -0.12 | -0.10 | -0.07 | -0.03 | 0.89 | 0.24 | 0.10 | 0.05 | 2.53  | 0.96 | 0.34 | 0.16 |
| MP2+CABS+LYP                   | -0.38 | -0.18 | -0.12 | -0.14 | 2.85 | 0.70 | 0.52 | 0.62 | 19.06 | 2.39 | 3.43 | 3.24 |
| MP2+CABS+TPSS                  | -0.33 | -0.14 | -0.08 | -0.03 | 0.88 | 0.25 | 0.11 | 0.05 | 3.05  | 1.06 | 0.35 | 0.17 |
| MP2+CABS+SCAN                  | -0.43 | -0.15 | -0.08 | 0.03  | 0.94 | 0.28 | 0.11 | 0.05 | 3.83  | 1.18 | 0.37 | 0.17 |
| MP2+CABS+PBE-CS ( $q = 1.88$ ) | -0.24 | -0.21 | -0.07 | -0.03 | 0.88 | 0.28 | 0.12 | 0.05 | 2.78  | 1.06 | 0.42 | 0.21 |
| MP2+CABS+PBE-HP ( $q = 2.05$ ) | -0.26 | -0.12 | -0.07 | -0.03 | 0.90 | 0.29 | 0.12 | 0.06 | 2.88  | 1.07 | 0.44 | 0.23 |
| MP2-F12                        | -0.28 | -0.10 | -0.03 | 0.00  | 0.31 | 0.13 | 0.03 | 0.00 | 1.38  | 0.54 | 0.09 | 0.00 |

[1] M. Schütz, R. Lindh and H.-J. Werner, Mol. Phys. **96**, 719 (1999).
